# Supplementary material for: Does Data Repair Lead to Fair Models? Curating Contextually Fair Data To Reduce Model Bias
Source: arXiv:2110.10389 source file (2021-10-20)
Supplement: Supplementary file 1 [file supple.tex]

\section{Curating Fair Data in Supervised Settings}
Following the experimental protocol of Section 5.1, in \cref{fig:representational_bias} we show the representational bias of the model at different selection budgets comparing with sampling techniques like \textit{Random} and \textit{Repair(Ranking)}. We can see that curating contextually balanced data using our approach helps in reducing the representational bias of the model. Further in \cref{tab:tpr_cup_supervised} and \cref{tab:ap_cup_supervised} we report per class true positive rate and average precision of each sampling technique at different budgets. 
\begin{figure}[h]
    \centering
    \includegraphics[height = 4cm, width = 6cm]{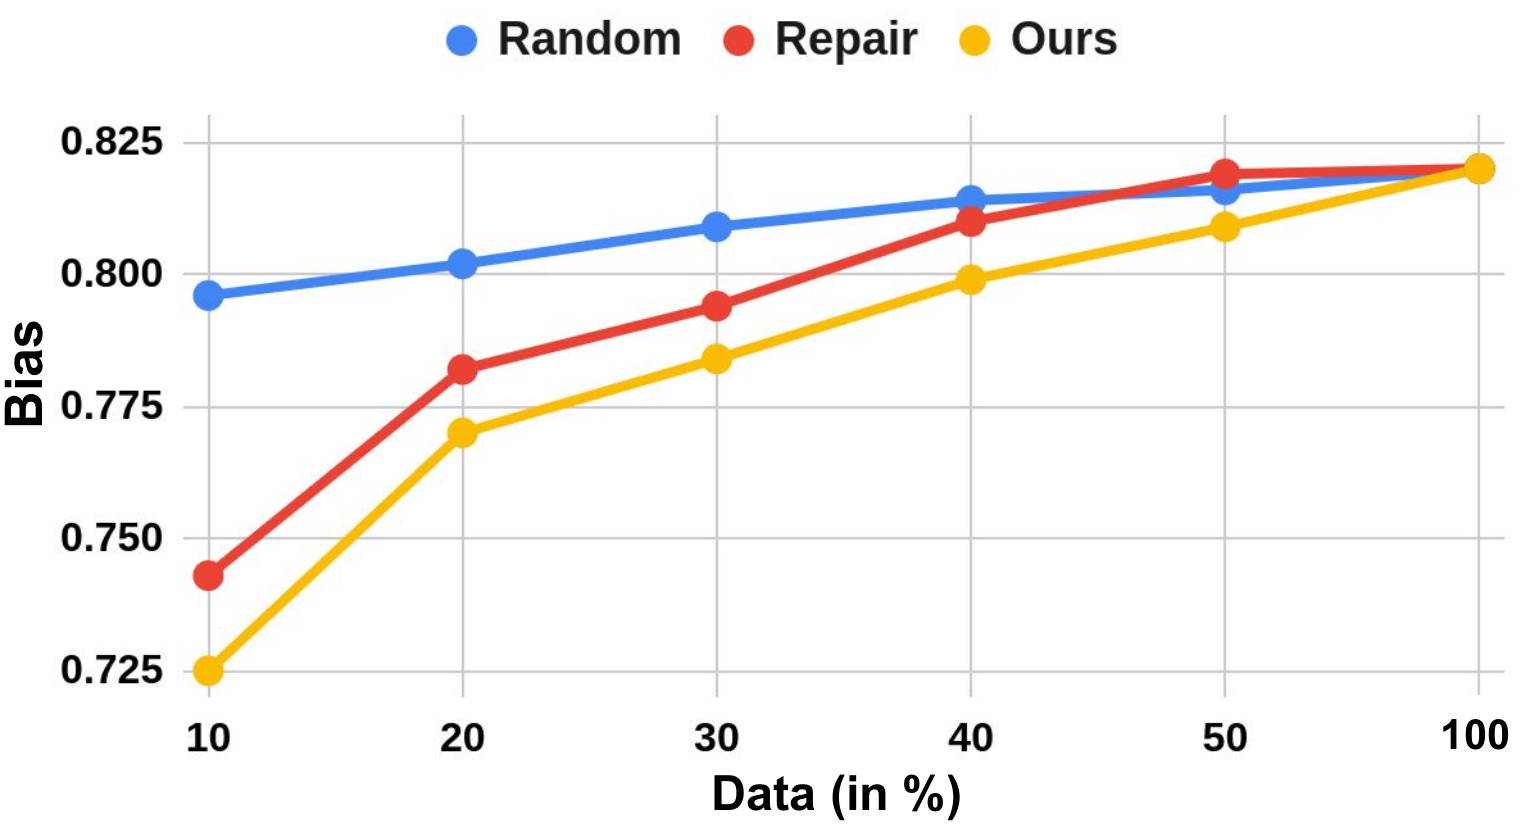}
    \caption{Representational Bias of the model in supervised setting}
    \label{fig:representational_bias}
\end{figure}
\section{Curating Data in AL setting with ALOFT}
\cref{tab:tpr_aloft} and \cref{tab:ap_aloft} reports per class true positive rate and average precision in active learning setting. Since, the reported results are average of three independent runs in  \cref{tab:eod_error} and \cref{tab:map_error} we report average score with standard errors.

\section{Curating Fair Data to Mitigate Gender Bias}
As discussed in Section 5.4, COCO suffers from gender bias with its 79 object categories. In \cref{fig:gender_stats} we plot the co-occurrence of male(blue) and female(red) with all 79 categories. We can see that males are biased in almost all the categories by a significant margin as compared to females, thus this contextual bias is important to be fixed for real-world application.

Further in \cref{tab:balanced_data} we report bias amplification $\Delta$, mAP and F1 score at different values of $\alpha$ in comparison with the selection heuristic proposed by balanced data[46]\footnote{citation number are in reference with main paper }. 

\begin{figure}
	\includegraphics[height = 4.5cm, width=\linewidth]{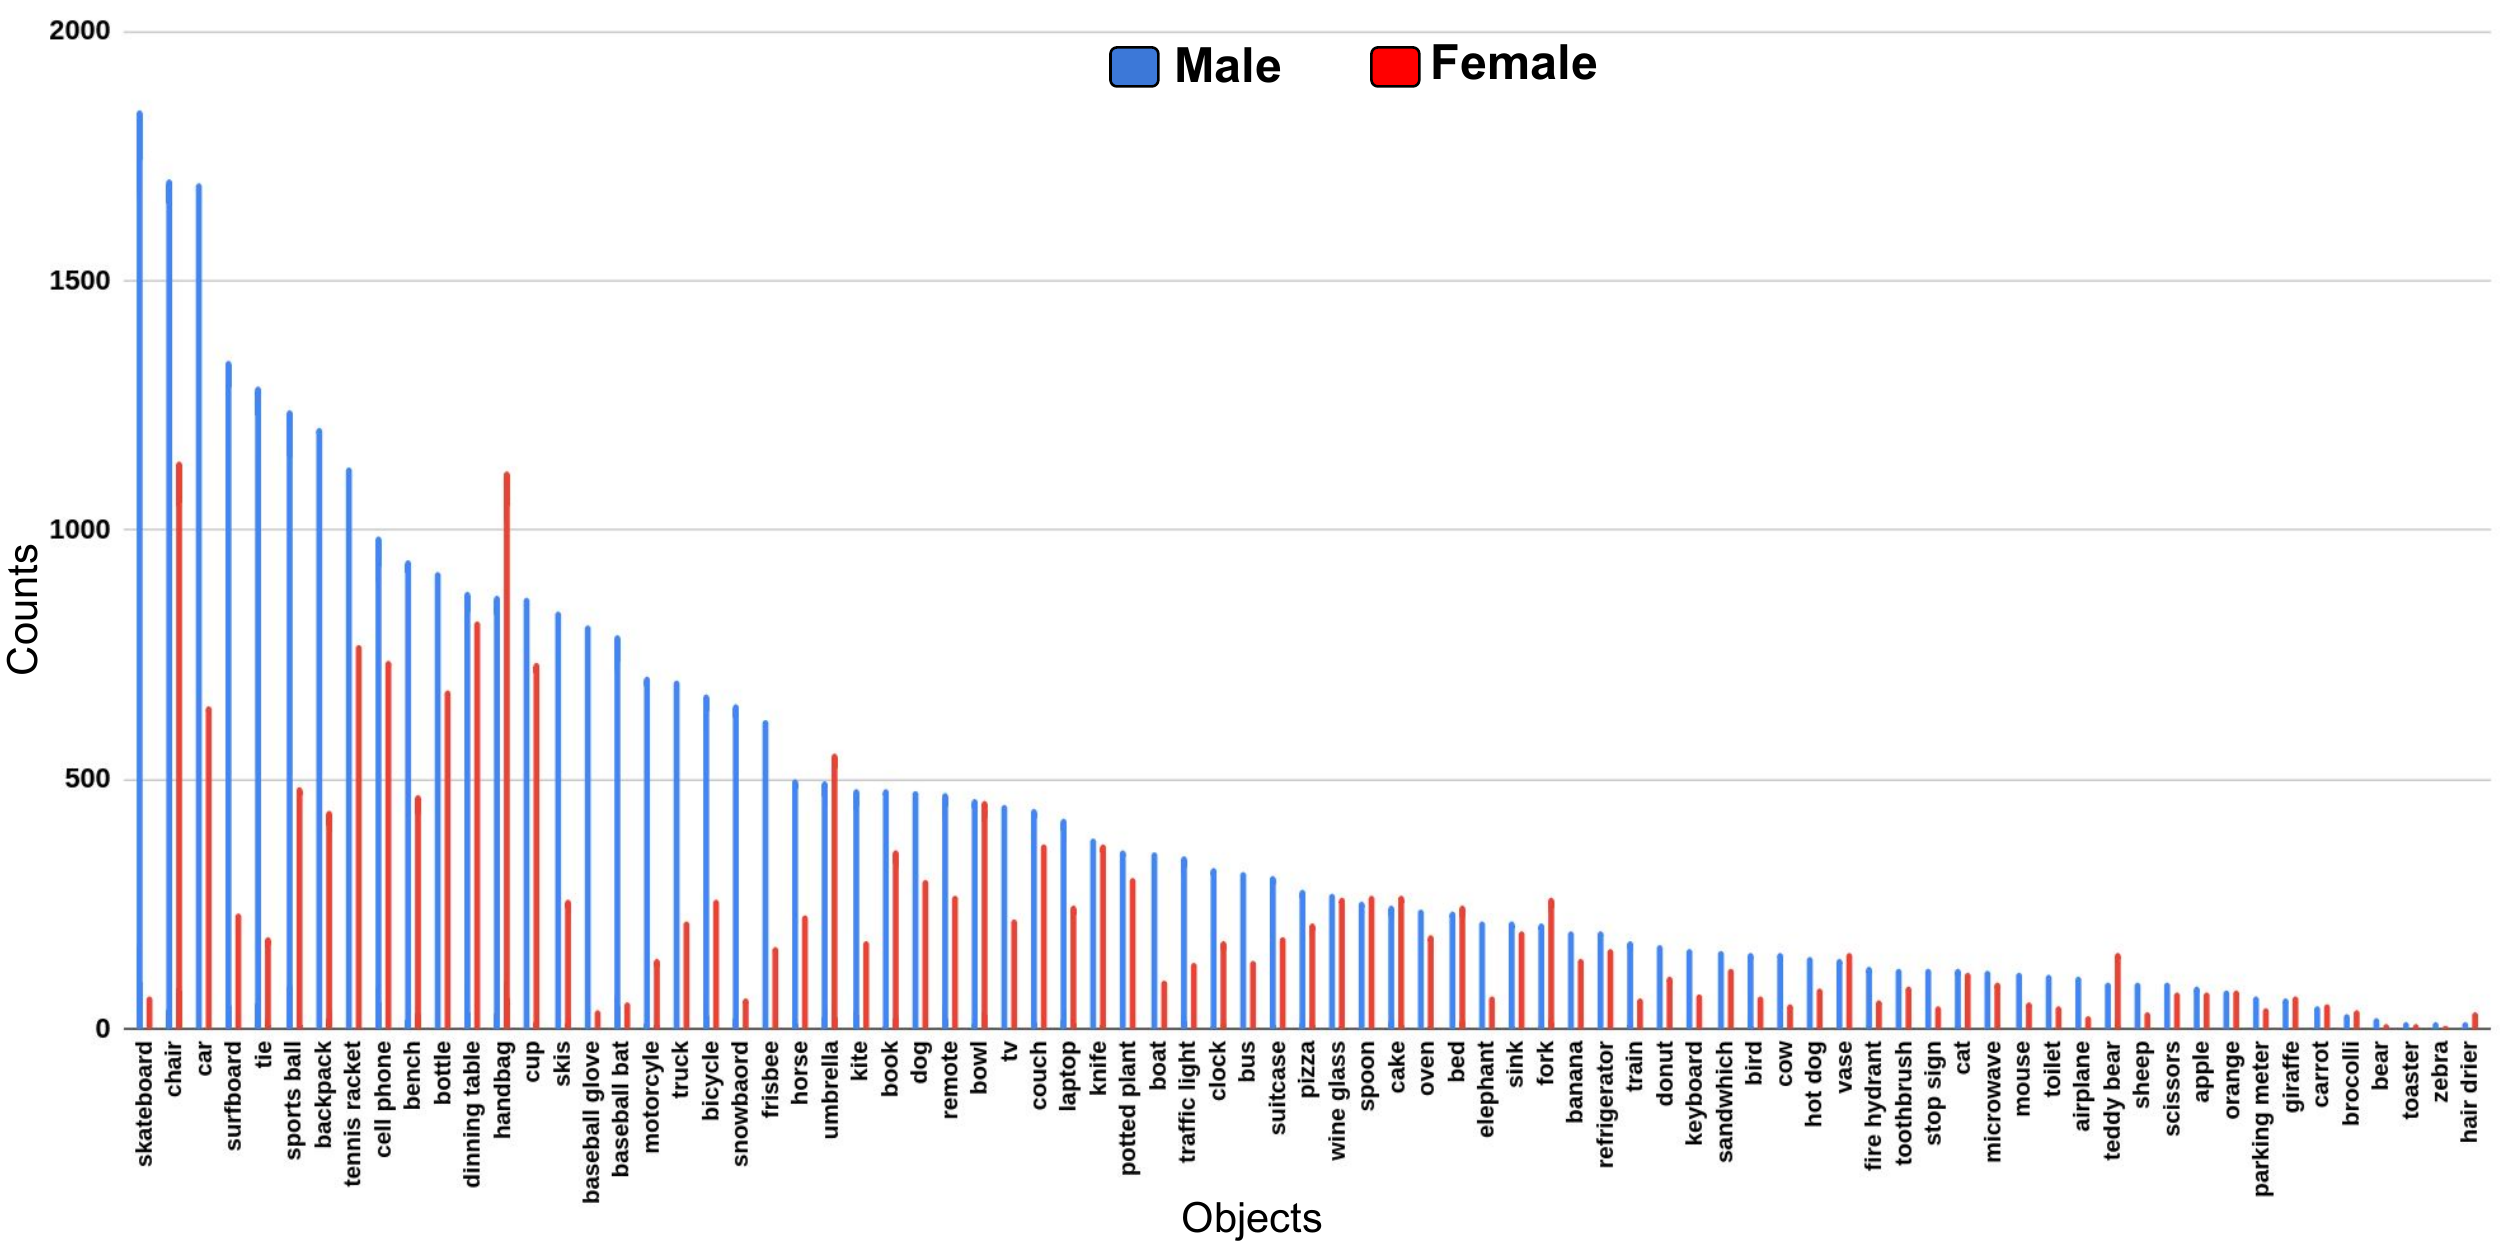}
	\caption{Contextual bias in COCO of 80 object categories with man and woman. Best visible at 6$\times$ zoom.}
	\label{fig:gender_stats}
\end{figure}

\subsection{Comparison with Soft Sampling Techniques}
Usually, standard object detection models are trained with cross-entropy loss, but many techniques have been proposed to handle data imbalance, like oversampling and soft sampling. Mostly oversampling leads to overfitting the model; thus, soft sampling techniques are preferred. We have used following soft sampling techniques for our analysis:

\begin{enumerate}[noitemsep]
	\item \textit{Class weighted cross entropy}, in this case the standard cross entropy loss is replaced by weighted cross entropy $CE(p_{s}) = -log(p_{s})$ where weights are defined as inverse of the class frequency. $WCE(p_s) = -\alpha log(p_{s})$, weighting factor $\alpha \epsilon[0,1]$
	\item \textit{Focal loss}[25] which dynamically assigns more weight to the hard samples. $FL(p_{s}) = -(1-p_{s})^\gamma \log(p_s)$, where $p_{s}$ is the estimation probability of the prediction and $\gamma$ is set as 2 to ensure a balance between hard and easy samples.
	\item \textit{Class Balancing loss}[10] where effective number of samples are used to assign weights for each class such that the loss is balanced to handle class imbalance.
\end{enumerate}

For this experiment we have selected categories like `skateboard', `surfboard', `sports ball', `tennis racket', `skis', `baseball glove', `baseball bat', `snowboard' and `frisbee' biased towards protected attribute `male' and `female'. The processed dataset consists of $2997$ and $621$ images of male and female respectively in training set with a $c_v$ of $0.5$ and $1.08$ respectively. 

We train ResNet50 on 20\% data curated randomly and using our approach from the available data balancing male and female across the $10$ selected contextual classes. The standard cross-entropy loss of the model was replaced with the above-mentioned soft sampling loss for both random and fair selection. We see in \cref{tab:soft_sampling} that with our fair selection model trained with cross-entropy loss achieved an mAP of 38.17, which is higher than the best performing weighted cross-entropy for random selection. Performance even improves when we replace the cross-entropy loss with the class balancing loss in our case. 

\begin{table}[h]
\footnotesize
\centering
\caption{Results of using soft sampling techniques to handle class imabalnce. We reoprt $c_v$ score of random and our selection with mAP of the classification model with each soft sampling loss. We can see using our sampling technique helps in boosting the model perforance when accompanied with class-balancing loss.}
\vspace{0.1cm}
\begin{tabular}{|c|c|c|c|}\hline
Method & Sampling & mAP $(\uparrow)$ & $c_v$(female)$(\downarrow)$  \\\hline
\multirow{4}{*}{Random} &Cross Entropy&36.28&\multirow{4}{*}{1.13}\\
&Weighted CE&37.7&\\
&Focal Loss&37.5&\\
&Class balancing loss&36.65& \\\hline
\multirow{4}{*}{Ours}&Cross Entropy&38.17&\multirow{4}{*}{\textbf{0.5}}\\
&Weighted(CE)&41.5&\\
&Focal Loss&40.3&\\
&Class balancing Loss & \textbf{42.75}&\\\hline
\end{tabular}
\label{tab:soft_sampling}
\end{table}

\begin{table}[h]
    \footnotesize
    \centering
    \caption{Average precision for the biased class in every biased pair. We show comparison between standard classifier trained using 100\% data over classifier trained on fairly curated data.}
    \vspace{0.1cm}
    \begin{tabular}{|c|c|c|c|c|c|}\hline
        \multicolumn{2}{c}{Classes} &\multicolumn{2}{c}{ Exclusive} & \multicolumn{2}{c}{Co-occur} \\\hline
         Bias & Co-occur & Stand. & Ours & Stand. & Ours \\\hline
         Cup & Din-Table & 79 & 82 & 88 & 94 \\
         WineGlass & Person & 78 & 96 & 88 & 95 \\
         Handbag & Person & 61 & 59 & 78 & 81 \\
         Apple & Fruit & 73 & 89 & 92 & 97 \\
         Car & Road & 75 & 86 & 87 & 93 \\
         Bus & Road & 91 & 93 & 93 & 97 \\
         Pot Plant & Vase & 82 & 85 & 91 & 94 \\
         Spoon & Bowl & 81 & 82 & 89 & 91 \\
         Microwave & Oven & 84 & 92 & 97 & 99 \\
         Keyboard & Mouse & 82 & 94 & 93 & 98 \\
         Skis & Person & 69 & 0 & 98 & 99 \\
         Clock & Building & 74 & 87 & 87 & 96 \\
         SportsBall & Person & 55 & 80 & 92 & 94 \\
         Remote & Person & 77 & 86 & 88 & 94 \\
         Snowboard & Person & 100 & 100 & 98 & 98 \\
         Toaster & Ceiling & 87 & 88 & 100 & 100 \\
         Hair Drier & Towel & 100 & 100 & 89 & 91 \\
         Tennisracket & Person & 100 & 100 & 94 & 98 \\
         Skateboard & Person & 100 & 100 & 86 & 96 \\
         Base-Glove & Person & 50 & 100 & 96 & 99\\\hline
         Average& &  80 & 85 & 91 & 95\\\hline
    \end{tabular}
    \label{tab:multilabel}
\end{table}

\section{Multi Label Image Classification}
For multi label image classification as discussed in Section 5.6 we perform fair selection over COCO for 20 biased pairs. In \cref{tab:multilabel} we show improvement in values of average precision for each biased class when it occurs exclusively or co-occur with the biased pair. We see that average precision in almost all the pairs has improved when the model is trained on fairly curated data in comparison to standard classifier trained with 100\% training data.

\section{Evaluation Metric}
In this section we briefly discuss bias amplification $\Delta:=\lambda_M-\lambda_D$, proposed by [46]. Bias amplification is defined as the difference between dataset and model leakage. 

\textbf{Dataset Leakage}:
is defined as a measure to estimate the protected attribute in presence of ground truth label. For a given image $X_i$ in dataset $D$, ($Y_i$,$g_i$) are defined as the ground truth label and protected attribute(male/female) respectively. Leakage is measured in terms of the information that attacker $f$ leaks in predicting $g_i$ through $Y_i$. Attacker $f$ tries to predict the protected attribute for image $X_i$ only using the task specific label $Y_i$, formally defining:
\begin{align}
    \lambda_{D} = \frac{1}{|D|}\sum_{Y_i,g_i}\mathbbm{1}[f(Y_i) == g_i]
\end{align}

\textbf{Model Leakage}: Similar to the dataset leakage, model leakage measures the leak in information by the model $M$ in predicting protected attribute $g_i$, for this case a different attacker is trained on $\hat{Y}_i$ to predict protected attribute $g_i$.
\begin{align}
    \lambda_M = \frac{1}{|D|}\sum_{\hat{Y}_i,g_i\in D}\mathbbm{1}[f(\hat{Y}_i)==g_i]
\end{align}

\begin{table*}[h]
	\centering
	\footnotesize
	\caption{In this table we report the true positive rate of predicting `Cup' in the presence of various contextual classes, in \textbf{supervised} setting.}
	\vspace{0.1cm}
	\begin{tabular}{|c|c|cccccccccc|c|}\hline
		Data(\%)& Method & Person & Din-Table & Bottle &Chair &Bowl & Knife & Fork & Spoon & Wine Glass & Sink & EoD $(\downarrow)$\\\hline
		\multirow{5}{*}{10} & Random & 0.53 & 0.56 & 0.47 & 0.58 & 0.45 & 0.52 & 0.6 & 0.54 & 0.35 & 0.29 & 0.1009  \\
		& Ranking & 0.51 & 0.55 & 0.45 & 0.56 & 0.45 & 0.51 & 0.6 & 0.53 & 0.36 & 0.27 & 0.1002  \\
		& Per-class rank & 0.51 & 0.52 & 0.45 & 0.55 & 0.42 & 0.44 & 0.54 & 0.5 & 0.25 & 0.25 & 0.11 \\
		& Threshold & 0.53 & 0.58 & 0.47 & 0.59 & 0.45 & 0.56 & 0.63 & 0.56 & 0.34 & 0.56 & 0.118 \\
		& Ours & 0.5 & 0.55 & 0.46 & 0.56 & 0.46 & 0.53 & 0.59 & 0.52 & 0.37 & 0.31 &\textbf{0.087}\\\hline
		\multirow{5}{*}{20}  & Random & 0.55 & 0.59 & 0.5 & 0.62 & 0.47 & 0.54 & 0.59 & 0.54 & 0.35 & 0.3 & 0.1051 \\
		& Ranking & 0.56 & 0.6 & 0.5 & 0.61 & 0.48 & 0.57 & 0.62 & 0.57 & 0.42 & 0.32 & 0.095 \\
		& Per-class rank & 0.52 & 0.55 & 0.44 & 0.56 & 0.42 & 0.53 & 0.6 & 0.49 & 0.32 & 0.24 & 0.114 \\
		& Threshold & 0.55 & 0.59 & 0.47 & 0.6 & 0.45 & 0.56 & 0.63 & 0.55 & 0.38 & 0.3 & 0.106 \\
		& Ours & 0.56 & 0.6 & 0.5 & 0.61 & 0.48 & 0.57 & 0.62 & 0.57 & 0.42 & 0.32 & \textbf{0.0959}\\\hline
		\multirow{5}{*}{30}  & Random & 0.56 & 0.61 & 0.49 & 0.62 & 0.49 & 0.56 & 0.64 & 0.57 & 0.38 & 0.32 & 0.1051\\
		& Ranking & 0.57 & 0.62 & 0.51 & 0.63 & 0.5 & 0.6 & 0.66 & 0.57 & 0.41 & 0.31 & 0.108 \\
		& Per-class rank & 0.58 & 0.58 & 0.49 & 0.61 & 0.47 & 0.54 & 0.6 & 0.52 & 0.34 & 0.25 & 0.118\\
		& Threshold & 0.6 & 0.64 & 0.53 & 0.64 & 0.52 & 0.65 & 0.69 & 0.62 & 0.46 & 0.38 & 0.098\\
		& Ours & 0.56 & 0.6 & 0.51 & 0.6 & 0.51 & 0.56 & 0.61 & 0.56 & 0.42 & 0.35 & \textbf{0.084}\\\hline
		\multirow{5}{*}{40}  & Random & 0.58 & 0.63 & 0.51 & 0.63 & 0.51 & 0.6 & 0.65 & 0.57 & 0.41 & 0.34 & 0.1017\\
		& Ranking & 0.59 & 0.63 & 0.54 & 0.65 & 0.52 & 0.62 & 0.68 & 0.57 & 0.45 & 0.33 & 0.1049 \\
		& Per-class rank & 0.57 & 0.58 & 0.49 & 0.61 & 0.46 & 0.55 & 0.61 & 0.54 & 0.34 & 0.28 & 0.113 \\
		& Threshold & 0.58 & 0.61 & 0.5 & 0.63 & 0.5 & 0.59 & 0.65 & 0.56 & 0.41 & 0.3 & 0.109\\
		& Ours & 0.57 & 0.61 & 0.52 & 0.62 & 0.53 & 0.59 & 0.63 & 0.57 & 0.42 & 0.39 & \textbf{0.082}\\\hline
		\multirow{5}{*}{50}  & Random & 0.61 & 0.65 & 0.55 & 0.66 & 0.53 & 0.62 & 0.68 & 0.62 & 0.43 & 0.35 & 0.1071 \\
		& Ranking & 0.6 & 0.63 & 0.52 & 0.64 & 0.53 & 0.6 & 0.68 & 0.58 & 0.44 & 0.33 & 0.1048 \\
		& Per-class rank & 0.59 & 0.6 & 0.51 & 0.63 & 0.5 & 0.57 & 0.63 & 0.56 & 0.37 & 0.27 & 0.118 \\
		& Threshold & 0.58 & 0.62 & 0.58 & 0.62 & 0.5 & 0.59 & 0.65 & 0.56 & 0.41 & 0.25 & 0.115 \\
		& Ours & 0.58 & 0.62 & 0.53 & 0.64 & 0.53 & 0.61 & 0.64 & 0.57 & 0.41 & 0.43 & \textbf{0.081}\\\hline
	\end{tabular}
	\label{tab:tpr_cup_supervised}
\end{table*}

\begin{table*}[h]
	\centering
	\footnotesize
	\caption{In this table we report per class average precision of the contextual classes in presence of the protected attribute `Cup' , in \textbf{supervised} setting.}
	\vspace{0.1cm}
	\begin{tabular}{|c|c|cccccccccc|c|}\hline
		Data(\%)& Method & Person & Din-Table & Bottle &Chair &Bowl & Knife & Fork & Spoon & Wine Glass & Sink & mAP$(\uparrow)$\\\hline
		\multirow{5}{*}{10} & Random & 60.5 & 33.5 & 37.43 & 25.56 & 27.78 & 8.11 & 16.24 & 12.33 & 26.5 & 13.06 & 26.1 \\
		& Ranking & 65.6 & 35.14 & 42.87 & 26.42 & 31.45 & 8.81 & 16.94 & 12.02 & 31.27 & 9.92 & 28.04 \\
		& Per-class rank & 62.5	&34.2&	37.5&	20.5&	30.6&	8.1&	11.6&	9.4&	28.36&	10.63 & 25.2  \\
		& Threshold & 61.5&	34.5&	37.43&	25.4&	28.78&	8.51&	16.24&	13&	25.5&	11.06 & 26.2 \\
		& Ours & 57.43 & 31.51 & 38.79 & 22.15 & 35.88 & 12.81 & 15.41 & 16.43 & 35.21 & 24.6 & \textbf{29.02} \\\hline
		\multirow{5}{*}{20} & Random & 65.25 & 38.41 & 43.58 & 25.14 & 45.06 & 14.32 & 26.28 & 15.25 & 27.78 & 24.32 & 32.53 \\
		& Ranking & 65.66 & 40.13 & 41.17 & 27.09 & 40.33 & 15.73 & 29.87 & 16.44 & 35.03 & 16.03 & 32.74 \\
		& Per-class rank &62.43&	30.51&	35.79&	22.15&	35.88&	11.81&	15.41&	17.43&	34.21&	22.6 &28.6 \\
		& Threshold &  64.66&	40.5&	40.4&	29.1	&41.43&	15.73&	29.37&	11.03&	30.03&	14.03 & 31.29 \\
		& Ours & 60.72 & 35.71 & 43.56 & 27.1 & 38.41 & 16.87 & 25.53 & 19.85 & 40.98 & 32.08 & \textbf{34.08} \\\hline
		\multirow{5}{*}{30} & Random & 69.6 & 41.02 & 46.21 & 33.28 & 38.65 & 24.41 & 34.81 & 20.13 & 34.97 & 31.57 & 37.46 \\
		& Ranking & 70.67 & 41.71 & 44.06 & 31.08 & 40.08 & 26.74 & 38.2 & 26.21 & 38.5 & 23.15 & 36 \\
		& Per-class rank &61.43&	30.51&	41.79&	23.15&	36.88&	17.81&	14.31&	15.43&	30.21&	23.69 & 29.8 \\
		& Threshold &  65.72&	32.71&	41.56&	27.1&	39.41&	15.87&	25.53&	19.85&	40.98&	32.08 & 34 \\
		& Ours & 66.22 & 39.29 & 44.5 & 26.23 & 36.77 & 24.65 & 35.19 & 26.85 & 41.57 & 33.47 & \textbf{37.47} \\\hline
		\multirow{5}{*}{40} & Random & 69.6 & 41.02 & 46.21 & 33.28 & 38.65 & 24.41 & 34.81 & 20.13 & 34.97 & 31.57 & 37.46 \\
		& Ranking & 70.67 & 41.71 & 44.06 & 31.08 & 40.08 & 26.74 & 38.2 & 26.21 & 38.5 & 23.15 & 38.04 \\
		& Per-class rank &  60.25&	35.41&	43.38&	21.14&	41.06&	15.92&	27.28&	15.25&	27.78&	21.32 & 30.6 \\
		& Threshold &  65.72&	37.71&	43.56&	28.1&	39.41&	15.87&	24.53&	22.85&	40.98&	31.08 & 34.9 \\
		& Ours & 64.2 & 40.69 & 45.12 & 29.89 & 39.59 & 20.18 & 40.78 & 26.27 & 47.78 & 37.48 & \textbf{39.19} \\\hline
		\multirow{5}{*}{50} & Random & 69.82 & 42.84 & 45.46 & 33.75 & 44.4 & 21.38 & 34.39 & 21.86 & 40.18 & 34.25 & 38.83 \\
		& Ranking & 69.66 & 43.83 & 45.2 & 31.5 & 42.89 & 26.12 & 42.95 & 23.83 & 42.19 & 23.92 & 39.5 \\
		& Per-class rank & 69.61&	39.92&	39.88&	30.49&	40.93&	18.76&	31.48&	20.81&	33.73&	24.75 & 35.5  \\
		& Threshold & 67.22&	39.29& 45.5&	26.23&	37.77&	26.65&	35.19&	27.85&	41.57&	30.47& 37.9 \\
		& Ours & 67.15 & 42.26 & 46.81 & 30.21 & 44.97 & 23.4 & 43.75 & 25.88 & 43.75 & 35 & \textbf{40.32}\\\hline
	\end{tabular}
	\label{tab:ap_cup_supervised}
\end{table*}

\begin{table*}[h]
	\centering
	\footnotesize
	\caption{In this table we report the true positive rate of predicting `Cup' in the presence of various contextual classes, in \textbf{Active learning} setting}
	\vspace{0.1cm}
	\begin{tabular}{|c|c|cccccccccc|c|}\hline
		Data(\%)& Method & Person & Din-Table & Bottle &Chair &Bowl & Knife & Fork & Spoon & Wine Glass & Sink & EoD$(\downarrow)$\\\hline
		10 & Random & 0.51 & 0.55&	0.45&	0.54&	0.44&	0.51&	0.57&	0.5&	0.31&	0.26&	0.1033   \\\hline
		\multirow{5}{*}{20} & Random &  0.54&	0.58&	0.46&	0.56&	0.45&	0.58&	0.63&	0.53&	0.34&	0.3&	0.1082  \\
		& Coreset & 0.47&	0.5&	0.42&	0.53&	0.4&	0.48&	0.54&	0.45&	0.27&	0.2&	0.111  \\
		& Max-Ent & 0.52&	0.55&	0.47&	0.58&	0.44&	0.52&	0.61&	0.5&	0.32&	0.27&	0.1089  \\
		& CDAL & 0.48&	0.51&	0.42&	0.56&	0.42&	0.47&	0.53&	0.45&	0.29&	0.22&	0.1062  \\
		& ALOFT & 0.46&	0.52&	0.41&	0.5&	0.42&	0.45&	0.52&	0.46&	0.34&	0.317&	\textbf{0.0711}\\\hline
		\multirow{5}{*}{30} & Random &  0.54&	0.59&	0.49&	0.59&	0.57&	0.54&	0.59&	0.55&	0.35&	0.3& 0.1013   \\
		& Coreset & 0.56&	0.58&	0.48&	0.61&	0.44&	0.58&	0.64&	0.52&	0.37&	0.25&	0.121 \\
		& Max-Ent & 0.53&	0.59 &0.46&	0.61&	0.46&	0.59&	0.67&	0.55&	0.367&	0.29&	0.1185 \\
		& CDAL & 0.53&	0.56&	0.48&	0.57&	0.45&	0.56&	0.65&	0.57&	0.35&	0.24&	0.1217  \\
		& ALOFT & 0.52&	0.56&	0.47&	0.56&	0.49&	0.52&	0.58&	0.53&	0.37&	0.37&	\textbf{0.0745}\\\hline
		\multirow{5}{*}{40} & Random &  0.53&	0.57&	0.47&	0.58&	0.47&	0.56&	0.63&	0.54&	0.33&	0.3&	0.108   \\
		& Coreset & 0.52&	0.56&	0.45&	0.59&	0.45&	0.53&	0.62&	0.53&	0.33&	0.22&	0.1232  \\
		& Max-Ent & 0.57&	0.59&	0.48&	0.6&	0.47&	0.55&	0.62&	0.51&	0.37&	0.27&	0.1111  \\
		& CDAL & 0.55&	0.58&	0.47&	0.62&	0.48&	0.56&	0.66&	0.59&	0.38&	0.23&	0.1281 \\
 		& ALOFT & 0.52	&0.57&	0.49&	0.56&	0.47&	0.54& 0.57&	0.48&	0.33&	0.34&	\textbf{0.0886}\\\hline
		\multirow{5}{*}{50} & Random &  0.53&	0.58&	0.49&	0.59&	0.47&	0.54&	0.6&	0.5&	0.33&	0.31&	0.1015   \\
		& Coreset & 0.56&	0.59&	0.5&	0.6&	0.48&	0.55&	0.61&	0.55&	0.34&	0.3&	0.1076  \\
		& Max-Ent & 0.54&	0.57&	0.45&	0.61&	0.47&	0.56&	0.63&	0.53&	0.36&	0.29&	0.1091  \\
		& CDAL & 0.56&	0.58&	0.48&	0.6&	0.47&	0.56&	0.63&	0.53&	0.36&	0.27&	0.1131  \\
		& ALOFT & 0.55&	0.57&	0.49&	0.59&	0.46&	0.53&	0.6&	0.54&	0.32&	0.34&	\textbf{0.0987}\\\hline
	\end{tabular}
	
	\label{tab:tpr_aloft}
\end{table*}

\begin{table*}[h]
	\centering
	\footnotesize
	\caption{In this table we report per class average precision of the contextual classes in presence of the protected attribute `Cup', in \textbf{Active learning} setting.}
	\vspace{0.1cm}
	\begin{tabular}{|c|c|cccccccccc|c|}\hline
		Data(\%)& Method & Person & Din-Table & Bottle &Chair &Bowl & Knife & Fork & Spoon & Wine Glass & Sink & mAP$(\uparrow)$\\\hline
		10 & Random & 58.1 & 35.3 & 34.4 & 16.8 & 33.2 & 9.12 & 12.5 & 7.12 & 27.6 & 6.5 & 23.7   \\\hline
		\multirow{5}{*}{20} & Random & 62.2 & 34.1 & 37.2 & 20.1 & 30.6 & 8.6 & 11.2 & 9.5 & 28.2 & 20.1 & 25.9  \\
		& Coreset & 66.5 & 32.1 & 38.5 & 27.5 & 32.2 & 8.1 & 17.5 & 15.6 & 34.5 & 4.1 & 27.3\\
		& Max-Ent & 65.6 & 35.6 & 41.5 & 28.6 & 37.3 & 15.2 & 24.2 & 16.3 & 37.4 & 4.2 & \textbf{30.2}  \\
		& CDAL & 65.3 & 35.2 & 41.2 & 28.6 & 38.2 & 11.6 & 25.3 & 13.8 & 35.4 & 5.6 & 29.6  \\
		& ALOFT & 60.9 & 33.5 & 38.5 & 17.6 & 34.6 & 13.6 & 28.6 & 13.9 & 34.6 & 16.8  & 29.1\\\hline
		\multirow{5}{*}{30} & Random & 63.6 & 37.6 & 40.2 & 23.6 & 37.6 & 11.4 & 17.4 & 15.9 & 33.4 & 22.1 & 29.8   \\
		& Coreset & 66.2 & 36.2 & 42.1 & 28.5 & 35.4 & 13.2 & 22.1 & 18.2 & 29.1 & 9.2 & 29.8  \\
		& Max-Ent & 63.4 & 35.2 & 41.2 & 24.2 & 40.2 & 16.2 & 29.7 & 20.8 & 28.2 & 7.1 & 30.3  \\
		& CDAL & 68.1 & 40.5 & 43.2 & 27.6 & 40.1 & 16.9 & 24.2 & 18.3 & 34.2 & 8.1 & \textbf{31.8}  \\
		& ALOFT & 65.5 & 31.6 & 36.4 & 18.6 & 39.4 & 14.2 & 35.8 & 14.7 & 33.4 & 28.6 & 31.3\\\hline
		\multirow{5}{*}{40} & Random & 65.2 & 36.3 & 10.2 & 28.2 & 37.2 & 16.5 & 27.4 & 17.5 & 29.6 & 21.3 & 31.6  \\
		& Coreset & 66.3 & 35.2 & 42.1 & 26.5 & 37.2 & 13.5 & 28.4 & 17.2 & 33.2 & 17.4 & 31.4 \\
		& Max-Ent & 65.3 & 36.3 & 44.2 & 25.2 & 39.2 & 13.5 & 32.2 & 17.2 & 37.4 & 19.4 & 32.7\\
		& CDAL & 61.3 & 32.3 & 40.3 & 27.2 & 33.3 & 14.2 & 30.2 & 19.4 & 35.3 & 38.5 & 32.9  \\
		& ALOFT & 67.5 & 39.5 & 45.2 & 27.3 & 36.5 & 16.4 & 33.4 & 23.9 & 34.8 & 17.4 & \textbf{33.7}\\\hline
		\multirow{5}{*}{50} & Random & 64.2 & 38.3 & 42.9 & 27.2 & 38.3 & 20.3 &25.2 &17.2 &33.9 & 27 & 33.1  \\
		& Coreset & 66.1& 34.2 &46.2&24 .2&	37.6&	17.5&	32.2 &19.1 &31.9&21.2	&32.7  \\
		& Max-Ent & 66.3 & 38.3 & 43.2 & 24.2 & 41.9 & 21.5 & 29.4 & 18.7 & 31.4 & 21.4 & 33.2   \\
		& CDAL & 65.3 & 36.3 & 44.2 & 21.3 & 39.4 & 13.6 & 30.4 & 15.2 & 34.2 & 29.4 & 32.5   \\
		& ALOFT & 65.6 & 39.4 & 43.4 & 25.4 & 37.3 & 23.5 & 30.4 & 17.4 & 33.4 & 37.3 & \textbf{34.9} \\\hline
	\end{tabular}
	\vspace{5cm}
	\label{tab:ap_aloft}
\end{table*}

\begin{table*}[t]
	
	\centering
	\caption{In this table we report the average mAP value of the model with the standard error in Active Learning setting, as the reported results are average of three independent runs. }
	\vspace{0.1cm}
	\begin{tabular}{|c|c|c|c|c|c|}\hline
		\backslashbox{Method}{Data(\%)} & 10 & 20 & 30 & 40 & 50 \\\hline
		Random & \multirow{5}{*}{21.04$\pm$7.3} & 27.8 $\pm$ 1.3 & 30.5$\pm$0.8&31.9$\pm$0.3&32.8$\pm$0.4\\
		Coreset & &28.7$\pm$1.6 & 31.2$\pm$1.1 & 33.1$\pm$0.6 & 32.7$\pm$0.3\\
		MaxEnt & &30.9$\pm$1.1 & 32.3$\pm$0.6 & 33.2$\pm$0.5 & 33.2$\pm$0.1\\
		CDAL & &30.2$\pm$0.7 &32.7$\pm$1.5&32.1$\pm$1.1&33.1$\pm$0.7\\
		ALOFT &  & 31.2$\pm$0.2 &32.4$\pm$0.5& 33.9$\pm$0.5 & 34.3$\pm$0.3\\\hline
	\end{tabular}
    \label{tab:map_error}
\end{table*}

\begin{table*}
	
	\centering
	\caption{In this table we report the average EoD score with the standard error in Active Learning setting, as the reported results are average of three independent runs. }
	\vspace{0.1cm}
	\begin{tabular}{|c|c|c|c|c|c|}\hline
		\backslashbox{Method}{Data(\%)} & 10 & 20 & 30 & 40 & 50 \\\hline
		Random & \multirow{5}{*}{0.098$\pm$0.012} & 0.11$\pm$0.007 & 0.11$\pm$0.002 & 0.105$\pm$0.002 & 0.105 $\pm$0.004\\
		Coreset & & 0.11$\pm$0.002 & 0.11$\pm$0.008 &0.111$\pm$0.13&0.105$\pm$0.002\\
		MaxEnt & &0.108$\pm$0.004&0.115$\pm$0.004&0.104$\pm$0.005&0.106$\pm$0.004\\
		CDAL & &0.101$\pm$0.007&0.116$\pm$0.006&0.105$\pm$0.02&0.109$\pm$0.005\\
		ALOFT &  & 0.083$\pm$0.01&0.084$\pm$0.007&0.093$\pm$0.004&0.098$\pm$0.0003\\\hline
	\end{tabular}
    \label{tab:eod_error}
\end{table*}

\begin{table*}
    \centering
    \caption{Bias amplification and $c_v$ tradeoff between our approach(rows 5-7) and balanced data[46] rows(1-4), row(4) reports results of adversarial debiasing over balanced selection for $\alpha=1$. Our selection approach makes significantly better selection with low $c_v$ resulting in low $\Delta$(bias amplification) of the model. Reported results are using ResNet-50 }
    \label{tab:balanced_data}
    \begin{tabular}{|c|c|c|c|c|c|c|c|c|}\hline
         Method & Split & \# men & \# women & $c_v(men)(\downarrow)$&$c_v(women)(\downarrow)$&$\Delta(\downarrow)$ & mAP$(\uparrow)$ & F1$(\uparrow)$ \\\hline
         \multirow{4}{*}{Balanced Data[46]} & $\alpha$=1 & 3078 & 3078 & 1.117 & 0.534 & 10.37 & 48.23 & 42.89 \\
         &$\alpha$=2 & 8885 & 6588 &0.938& 1.036 & 9.73 & 56.21 & 51.95 \\
         & $\alpha$=3 & 10876 & 6598 &0.904& 1.035 & 10.23 & 57.04 & 52.6 \\
         &adv $@$conv$5$ & 3078 & 3078 & 0.953 & 1.035 & 2.51 & 43.71 & 38.98\\
         \hline
         \multirow{3}{*}{Ours} & $\alpha$=1 & 3646 & 2510 &\textbf{0.231}&\textbf{0.346}& \textbf{2.3} & 48.9 & 42.6 \\
         &$\alpha$=2 & 10114 & 5359 &0.767&0.365& 6.6 & 51.9 & 47.3 \\
         & $\alpha$=3 & 11649 & 5825 & 0.656 & 0.852 & 6.4 & 52.74 & 47.6 \\\hline
         Original & - & 16225 & 6601 & 0.953 & 1.035 & 9.93 & \textbf{58.23} & \textbf{53.75} \\\hline
    \end{tabular}
\end{table*}
